# Supplementary material for: Synchronization of Coupled Kuramoto Oscillators under Resource Constraints
Source: arXiv:2002.04092 ancillary file (2020-12-07)
Supplement: Supplementary file 1 [file ResourceConstrainedKuramotoPaperSupplement.pdf]

# Supplemental Information

## 1 Derivation of $|\omega_i - \Omega| < Kr$

We begin with the phase equation

$$\dot{\phi}_i = \omega_i + \frac{K}{N} \sum_j \sin(\phi_j - \phi_i)\,. \tag{1}$$

Consider just the summation over the sine term: we use Euler's identity to rewrite the sine as an exponential so that we have

$$\sum_j \sin(\phi_j - \phi_i) = \sum_j \frac{1}{2i}\left(e^{i\phi_j}e^{-i\phi_i} - e^{-i\phi_j}e^{i\phi_i}\right). \tag{2}$$

This then simplifies to

$$\frac{1}{2i}e^{-i\phi_i}\sum_j e^{i\phi_j} - \frac{1}{2i}e^{i\phi_i}\sum_j e^{-i\phi_j}\,. \tag{3}$$

The full summation of $e^{i\phi_j}$ is the definition of the order parameter $r$. That is,

$$\sum_j e^{i\phi_j} = Nre^{i\psi}\,. \tag{4}$$

Thus, equation 3 simplifies to

$$\frac{r}{2i}\left(e^{i(\psi-\phi_i)} - e^{-i(\psi-\phi_i)}\right) \tag{5}$$

which we can then simplify using Euler's identity to

$$r\sin(\psi - \phi_i)\,. \tag{6}$$

The phase velocity equation then becomes

$$\dot{\phi}_i = \omega_i + \frac{Kr}{N}\sin(\psi - \phi_i)\,. \tag{7}$$

We now note that the average velocity of the system is

$$\frac{1}{N}\sum_i \dot{\phi}_i = \frac{1}{N}\sum_i \left(\omega_i + \frac{K}{N}\sum_j \sin(\phi_j - \phi_i)\right). \tag{8}$$

Since $\sin(\phi_j - \phi_i)$ is antisymmetric, summing over both $i$ and $j$ will cause the second term to be zero. Thus, the average velocity is just the average internal velocity, and since we assumed that internal velocities could be considered approximately constant on the timescale of interest, we can assume the same here, meaning that the average velocity is constant. Since the average velocity is constant, denote it by $\Omega$. Then the time evolution of $\psi$ will be given by $\psi(t) = \Omega t + \psi_0$. We can then arbitrarily rotate our coordinate system so that $\psi_0 = 0$. Thus,

$$\dot{\phi}_i = \omega_i + \frac{Kr}{N}\sin(\Omega t - \phi_i)\,. \tag{9}$$

Now we go into a rotating coordinate system such that $\dot{\phi}_i \to \dot{\phi}_i + \Omega$, which means that $\phi_i \to \phi_i + \Omega t$. Carrying this through, we find

$$\dot{\phi}_i = \omega_i - \Omega - \frac{Kr}{N}\sin(\phi_i) \tag{10}$$

where now $\dot{\phi}_i$ is defined by the difference between the velocity of oscillator $i$ and the group velocity.

If oscillator $i$ is going to be captured by the group, it must be that the velocity of oscillator $i$ is equal to the group velocity, which means $\dot{\phi}_i = 0$ in this rotating coordinate frame. Further, the largest in magnitude that $\sin(\phi_i)$ can possibly be is 1, so the condition on synchronization being possible is that $\mu R_i - \Omega$ be less in magnitude than the largest value of the sine term. That is,

$$|\omega_i - \Omega| < \frac{Kr}{N}\,. \tag{11}$$

# 2 Derivation of Steady-State Order Parameter

Beginning now with the $\dot{\phi}_i$ equation from the previous section, we have

$$\dot{\phi}_i = \omega_i - \Omega - Kr\sin(\phi_i)\,. \tag{12}$$

Suppose we consider a system of infinite size. In the infinite-size limit the ratio $\frac{d_i}{N} = p$ where $p$ is the edge probability. This is a consequence of the central limit theorem. Further, in the infinite limit we can assume the system reaches a precise steady-state, as opposed to finite-sized systems where noise will always be present. Thus, for an oscillator in the infinite system we have

$$\dot{\phi}(\phi, \omega) = \omega - \Omega - Kr\sin\phi\,. \tag{13}$$

We can define a continuity equation for the density of oscillators $\rho(\phi, \omega)$ on $\phi \in [0, 2\pi)$ by

$$\frac{\partial \rho}{\partial t} + \frac{\partial}{\partial \phi}\big(\dot{\phi}\rho\big) = 0\,. \tag{14}$$

We assume that we have reached a steady-state so that $\frac{\partial \rho}{\partial t} = 0$, giving,

$$\frac{\partial \rho}{\partial \phi} = \frac{\rho}{\dot{\phi}}\frac{\partial \dot{\phi}}{\partial \phi}\,. \tag{15}$$

Plugging in $\dot{\phi}$, we have

$$\frac{\partial\rho}{\partial\phi} = \rho\frac{Kr\cos\phi}{\omega - \Omega - Kr\sin\phi}\,. \tag{16}$$

Thus,

$$\ln\rho = -\ln\left|\frac{\omega - \Omega - Kr\sin\phi}{Kr}\right| + C \tag{17}$$

which means

$$\rho(\phi,\omega) = A(\omega)\left|\frac{Kr}{\omega - \Omega - Kr\sin\phi}\right| \tag{18}$$

where we note that the constant of integration in $\phi$ could itself be a function of $\omega$.

Now suppose we know that the distribution of natural frequencies is $g(\omega)$. Thus, when we marginalize $\rho$ over $\phi$, we should obtain $g(\omega)$. However, notice that, as it stands, for values of $\omega$ where the denominator can diverge, the integral from 0 to $2\pi$ fails to converge. The only degree of freedom we have to fix this is the scaling factor $A(\omega)$. Thus, to force the integral to converge, we must take the limit as $A(\omega) \to 0$. In this limit, all of the finite components of $\rho(\phi,\omega)$ will go to zero, while the divergent components will remain infinite. This property is characteristic of the Dirac delta distribution. Additionally, there are actually two distinct points in $\phi$ where $\rho$ diverges. However, one of these is an unstable equilibrium, so the measure of the set of initial conditions that begin at that point is zero. Thus, we suppose that no oscillators are present at that point in the steady-state. Thus, for capturable values of $\omega$, we have

$$\rho(\phi,\omega) = g(\omega)\delta\left(\phi - \sin^{-1}\left(\frac{\omega - \Omega}{Kr}\right)\right) \tag{19}$$

where the range of $\sin^{-1}(x)$ is taken to be $[-\frac{\pi}{2}, \frac{\pi}{2}]$.

What about the oscillators that are not capturable? The quantity we are particularly interested in is the order parameter. Since $\psi = 0$ in our coordinate system, the order parameter is defined by

$$r = \int d\phi\, d\omega\, \rho(\phi,\omega)\cos(\phi)\,. \tag{20}$$

Notice now that the cosine is odd under the transformation $\phi \to \pi - \phi$. On the other hand, $\rho(\phi,\omega)$, which is a function only of $\sin\phi$, is even under that transformation. Thus, the integral will vanish by symmetry. The reason that this argument fails in the capturable case, incidentally, is because the instability of the second fixed point breaks the symmetry in the steady-state.

Thus, the order parameter of the system will be contributed to only by the capturable oscillators, whose distribution is given in equation (19). Let us now evaluate the order parameter:

$$r = \int d\phi\, d\omega\, g(\omega)\delta\left(\phi - \sin^{-1}\left(\frac{\omega - \Omega}{Kr}\right)\right)\cos\phi\,. \tag{21}$$

We can easily evaluate the $\phi$ integral and obtain

$$r = \int d\omega\, g(\omega) \cos\left( \sin^{-1}\left(\frac{\omega - \Omega}{Kr}\right)\right) \tag{22}$$

where the integral only runs over the values of $\omega$ which are capturable. That is, the bounds are $\omega = \Omega - Kr$ to $\omega = \Omega + Kr$. Making the substitution $\omega' = \frac{1}{Kr}(\omega - \Omega)$, the above equation becomes

$$r = Kr \int_{-1}^{1} d\omega'\, g\Big(Kr\omega' + \Omega\Big) \cos(\sin^{-1}(\omega'))\,. \tag{23}$$

Now shift the zero of $g(R)$ so that we can ignore the $\Omega$ term in the argument. That is $g'(Kr\omega') \equiv g(Kr\omega' + \Omega)$. Finally, we make a trig substitution so that $\omega' = \sin\omega''$. Then $d\omega' = \cos\omega'' d\omega''$. Our integral finally becomes

$$r = Kr \int_{-\frac{\pi}{2}}^{\frac{\pi}{2}} d\omega''\, g'(Kr\omega'') \cos^2(\omega'')\,. \tag{24}$$

Up to relabelings of primed variables to unprimed variables, this is the equation referenced in the paper.

# 3 Why Order Can (and Will) Increase

Suppose we have a finite-sized system with two steady-state solutions according to Equation (24). One of these solutions, suppose, is at $r = r_0$, and the other is at some larger value $r = r_1$. Broadly speaking, we can divide all of our oscillators into two groups at any order parameter which is reasonably steady over time. Some of the oscillators will be members of a group that moves as one unit and accounts for the steady component of the order parameter, and the rest of the oscillators will be uncaptured by that group and will thus pass by the group transiently, sometimes increasing order and sometimes decreasing it, thereby contributing noise to the order parameter. Importantly, these uncaptured oscillators have (dominantly) uncorrelated phases with respect to one another.

For an infinite-sized system, the contribution of the uncaptured oscillators to the order parameter, due to the uncorrelated phases of each uncaptured oscillator, would average out to zero, which is why noise in the order parameter vanishes in the thermodynamic limit. However, in a finite-sized system, there is always a finite-sized chance that many of the uncaptured oscillators find themselves in phase with the synchronized group at the same time, thereby momentarily increasing the order parameter of the system. The important difference between the $r_0$ state and the $r_1$ state is that the size of the captured subset of oscillators in the $r_0$ state is smaller than the size of the captured subset in the $r_1$ state. However, there is always a finite chance that, given we're in the $r_0$ state, all of the uncaptured oscillators in the $r_0$ state that are captured in the

$r_1$ state happen to be in phase with the synchronized group. If this happens, since the $r_1$ state is also a stable state, the system will then evolve in the $r_1$ state rather than the $r_0$ state. Further, since that subset of oscillators is now captured, the phases of all of those oscillators are no longer uncorrelated. Thus, the probability of going to the $r_0$ state from the $r_1$ state is zero.

The upshot of the above argument is that, for a finite-sized system, there is always a probability of transitioning from the lower-order state to the higher-order state in a bistable configuration. However, the probability of the reverse transition is zero. Thus, after an infinite time, any finite-sized bistable system is actually only meta-stable at the lower-order state, and only the higher-order state is truly stable. However, we can approximate the probability of the transition and see that the transition is indeed very unlikely over the course of a single simulation.

Suppose that in time $\Delta t$ the phases of all of the uncaptured oscillators sufficiently randomize so that we can consider a discrete-time process rather than a continuous-time one. Suppose a system of $N$ oscillators is bistable according to equation (24) with a stable state $r_0$ consisting of $N_0$ captured oscillators and another stable state $r_1$ consisting of $N_1$ captured oscillators, with $r_1 > r_0$ and therefore $N_1 > N_0$. Given the argument previously presented, the system will spontaneously transition from $r_0$ to $r_1$ if $N_1 - N_0$ oscillators happen to be in phase with the synchronized group at the same time. In fact, the condition is probably considerably weaker because if a sizable fraction of the $N_1 - N_0$ oscillators are in phase, it is likely that the remaining oscillators will come into phase faster than the in-phase oscillators go out of phase. However, since this argument is only approximate, suppose it really requires all of the oscillators to be in phase simultaneously. Further, "in phase" just means that the oscillators are within $\frac{\pi}{2}$ of the center of the synchronized group, so that if a given oscillator is closer to the center of the synchronized group than it is to the point on the opposite side of the circle, we will suppose it increases the order parameter by $1/N$, and if it's closer to the opposite point, it decreases the order parameter by $1/N$. That means that each oscillator just has to be in the correct half of the allowed phase space, which simplifies the math considerably. Thus, for each oscillator, in each time interval $\Delta t$ there is probability $p = \frac{1}{2}$ that the oscillator will be in phase with the synchronized group. Thus, the probability that all $N_1 - N_0$ oscillators will be in phase is $(\frac{1}{2})^{N_1 - N_0}$. We are interested in what the first moment is, on average, that all of the oscillators are in phase, so that the system transitions from $r_0$ to $r_1$. The reason we are interested in this moment when the system first transitions, rather than something like the probability of it being in one state versus the other, is that it will always *eventually* transition. In terms of an analagous energy landscape, it's as if there is a marble in a bowl sitting on a table getting jostled around constantly. It will definitely *eventually* jostle out of the bowl, and once it does, there's no way it's going to bounce back up off of the floor and back into the bowl. Thus, the question we're interested in is just how long on average it takes for the marble to wind up on the floor. To this end, let us calculate the number of steps it takes for the system to have a 50 percent chance of having transitioned. We are then interested in $P$(has not

transitioned at step $n$). This is just $P = (1 - (\frac{1}{2})^{N_1 - N_0})^n$. We are interested in when this probability is equal to 0.5. That is,

$$0.5 = \left(1 - \left(\frac{1}{2}\right)^{N_1 - N_0}\right)^{n_{\frac{1}{2}}} . \tag{25}$$

We can solve this equation for $n_{\frac{1}{2}}$, and we find

$$n_{\frac{1}{2}} = \frac{-\ln 2}{\ln\left((1 - (\frac{1}{2})^{N_1 - N_0})\right)} . \tag{26}$$

Since $\left(\frac{1}{2}\right)^{N_1 - N_0} \ll 1$, we can Taylor expand the denominator to first order and we find

$$n_{\frac{1}{2}} \approx 2^{N_1 - N_0} \ln 2 . \tag{27}$$

This means that, since each time step is length $\Delta t$,

$$t_{\frac{1}{2}} = \Delta t n_{\frac{1}{2}} \approx 2^{N_1 - N_0} \ln 2 \Delta t . \tag{28}$$

If we suppose that $r_0$ is at or near disorder, so that $N_0 \approx 0$, and that $r_1$ is a state with about half of the oscillators captured so that $N_1 \approx \frac{N}{2}$, given a system of 400 oscillators, as in our main paper, we have

$$t_{\frac{1}{2}} \approx 2^{200} \ln 2 \Delta t \approx 10^{60} \ln 2 \Delta t . \tag{29}$$

Thus, unless $\Delta t$ is infinitessimally small, the half-life of the metastable state is enormous, which is why we observe the system to be effectively bistable.

The other upshot of this metastability is that, given a line of stable points that are all relatively close together, the system will gradually march up that line to the largest available stable point, with the logarithm of the transition time between each point roughly proportional to the difference in the sizes of the stable groups. This explains why, given a line of stable points, the system will actually be observed at the largest stable point on the line, even if Equation (24) tells us that other stable points exist. Thus, the "close enough" referred to in the paper refers to the size of $t_{\frac{1}{2}}$ becoming small enough between the two stable points that a transition is likely to be observed in the course of the simulation. Determining *precisely* how close that is actually proves quite a challenge because $\Delta t$ is difficult to determine in practice, but we can see that at least the scaling behavior makes sense.

As a simple test, we supposed that, as long as the frequency distribution is the same, the "barrier" should be the same. However, as system size increases, the number of oscillators that must come together to overcome the barrier will increase in proportion. Thus, we initialized a simple Kuramoto system with a weakly bimodal distribution, shown by Pazo et al to produce bistability, in an unsynchronized state and let the simulation run until the system transitioned to its synchronized state. We then measured the average elapsed time for this to occur for varying system sizes. According to our theory above, this time should grow exponentially (though perhaps not with base 2, as suggested above, due to the considerable simplifications made in that presentation). Shown in Figure 1 is the growth of the transition time versus system size.

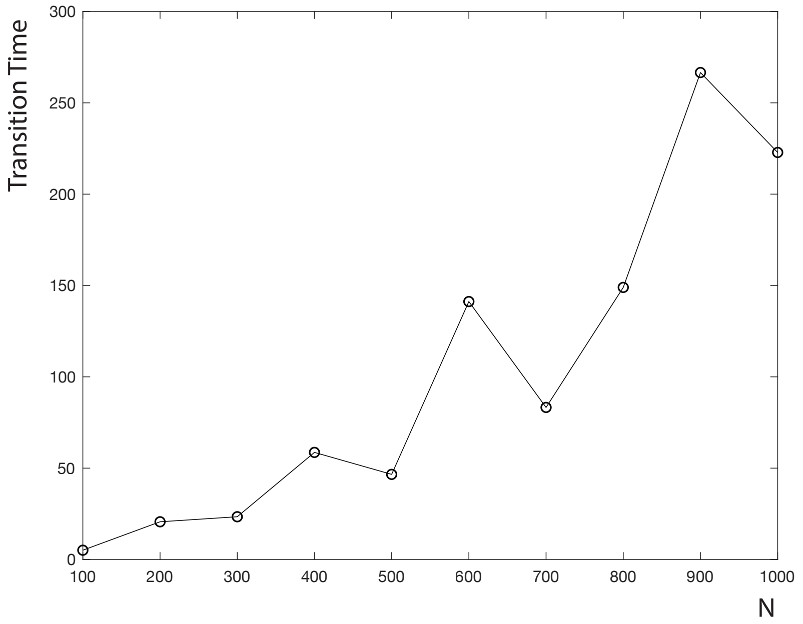


Figure 1: **Time before synchronization versus System size**.

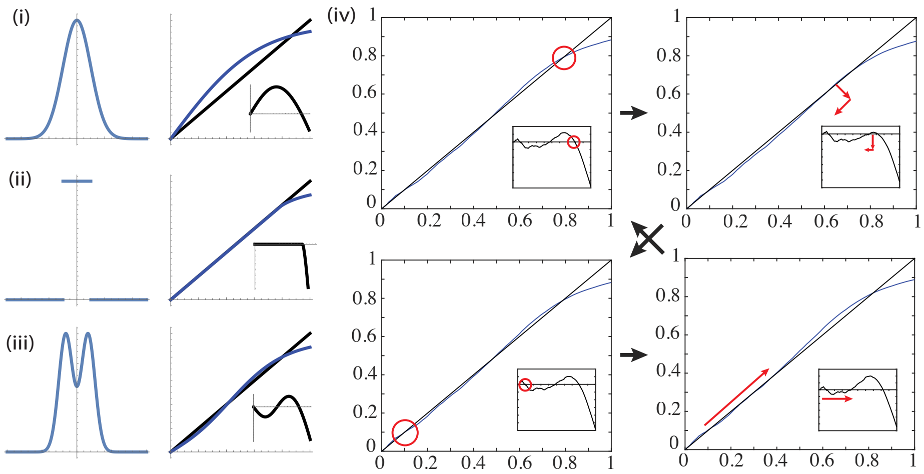


Figure 2: **Understanding Order Parameter Evolution.** Panels (i-iii) show sample resource level distributions and corresponding graphical solutions to $r = Kr \int d\omega \, \cos^2(\omega) g'(Kr\omega)$. The difference between the two sides of the equation can be interpreted as defining a dynamical system, which is inset in the bottom right. In (iv) we plot the right side of the equation in blue at four different moments of time over the evolution of our system.

# 4 One Dimensional Bifurcation Sequence

We mention in the main paper that the behavior of our system can be explained by a fast phenomenon, the phase synchronization, which behaves roughly as a one dimensional dynamical system with a set of parameters, and a slow phenomenon that essentially performs a parameter sweep over those parameters. For certain values of the parameters, there are bifurcations in the dynamical system, and so we see interesting behaviors arise as a result of the coupling between the value of the order parameter, defined by the dynamical system and the values of the parameters at a given time, and the slow drift of those parameters, defined by the motion toward a new equilibrium resource state. Here we will spell out these relationships in greater depth.

Consider Figure 2, which looks at the order parameter as a function of the resource distribution for our oscillatory behavior. We see that a Gaussian distribution has an unstable low-order solution and a stable high-order solution. A uniform distribution has a line of meta-stable solutions. Finally, a bimodal distribution has two stable solutions at low and high order and one unstable solution at intermediate order. Turning to (iv), where we plot the right side of the equation for our real resource distribution at different moments in time, we can use the (ii) and (iii) to interpret the behavior. Beginning in the top left of (iv), we are at a moment of high order, indicated by the red circle. We see that the dynamical system at this moment is very similar to that of the bimodal

distribution in (iii), and indeed we have discussed in the paper how bimodality arises in our system. When the order is high, the resource levels tend to move away from the mean value. This causes the peaks to drift outward and the trough in the center to lower. At some point, the high order solution to the dynamical system will vanish, as we see in the top right plot. At this moment, the order will quickly decrease down to what is, now, the only stable point. This will cause the movement of the resource levels to reverse, and so the shape of the dynamical system will gradually approach what it was in the top right. This is what we see in the bottom left plot. However, as a result of the bistability of this dynamical system, the order in the system will remain low even though the high-order solution has very quickly reappeared. As the resource levels drift closer together, the central part of the resource distribution will flatten out as it rises. Thus, the central region becomes somewhat uniform locally, though two peaks are still present on either side. The uniformity gives rise to the rough line of solutions seen in the bottom right plot, where the order of the system begins to increase again. The continued existence of the two peaks is evidenced by the fact that the line of solutions culminates in a large arc above the axis that then turns around, crosses the axis at the high order solution, and passes below to infinity. We see that this feature is absent in the simpler uniform distribution of (ii), where the line of solutions appears, but lacks the arc above the axis.

Reframing the above sequence in the language of bifurcation theory, we begin in a bistable system at the larger stable solution. The parameters then drift such that a saddle bifurcation occurs and the higher order solution vanishes. The system then only has a single fixed point at low order, so the order parameter quickly moves to that new value. The parameters then drift in reverse and the saddle bifurcation reoccurs at the higher order solution. However, due to the bistability, the value of the order parameter doesn't change. The parameters continue to drift in this reversed direction until a number of saddle bifurcations occur between the unstable intermediate-order solution and the stable low-order solution. As a result of the discussion in Section 3, the finite-sized system will jump upward along this line of closely-spaced solutions until it rises to the highest-order solution. The drift of the parameters will then reverse again and all of those new intermediate solutions will vanish, leaving the system back in a bistable state with the order parameter at the larger-order solution. We remain uncertain whether, in an infinite-sized system, where the considerations of Section 3 no longer apply, a true line of metastable solutions will appear as in subplot (ii) of Figure 1, or whether instead the intermediate unstable solution will continually approach the low-order solution until a subcritical pitchfork bifurcation occurs and the stable and unstable solutions join to form a single unstable solution. The latter case seems to us the more likely.

## 5 Bistability vs. Oscillations

We next turn to the question of what causes bistability in the one case versus oscillations in the other. We can understand this quite simply. If we consider

an oscillator which tends to have a higher resource level than average, and thus turns faster than the group on average, and if $\beta$ is chosen such that higher frequency results in greater resource consumption, then there exists a value of the effective coupling strength such that the oscillator will oscillate between capture and escape. This is because when the oscillator is captured, its frequency decreases to the slower group velocity, reducing its resource consumption, causing its resource level to rise, which then causes it to escape. Upon escaping, the oscillator turns faster, consuming additional resources, causing its resource level to fall, which then causes it to be captured again. Because the phase velocity can only take on one of essentially two states, and because neither state is stable, the oscillator will transition indefinitely.

On the other hand, suppose $\beta$ is chosen such that higher frequency results in greater resource production. In that case, when captured by the group, the oscillator will turn slower on average, thereby producing less resources, causing its resource level to fall, and so reinforcing its capture by the group. By the same token, if it were to somehow escape from the group, its frequency will increase, causing additional resource production, thereby increasing its resource level and reinforcing its independence from the group.

Thus, when oscillators consume resources as a function of their frequency, oscillations occur, and when oscillators produce resources as a function of their frequency, bistability occurs. However, given identical oscillators, only one or the other behavior will occur. The behavior of mixed populations of producing and consuming oscillators remains an open question.

# 6 Simplifying the Dynamical System

Much of the discussion in the main paper is based on developing and verifying intuition regarding the observed behaviors. However, mathematical rigor is not presented there. Here we will use the Ott-Antonsen (2017) ansatz and a two-timing approximation to obtain a more simplified set of dynamical equations describing the behavior in the thermodynamic limit. However, these equations remain difficult to work with, and did not provide us any further insight. Nonetheless, we present them here for the interested reader.

We begin with the dynamical equation defining the system:

$$\dot{\phi}_i = \omega_i + \frac{K}{N}\sum_j \sin(\phi_j - \phi_i) \tag{30}$$

$$\dot{\omega}_i = D(\Omega_i - \omega_i) + \beta\frac{K}{N}\sum_j \sin(\phi_j - \phi_i). \tag{31}$$

The state of the system is then defined by a probability distribution $\rho(\phi, \omega, \Omega; t)$. The continuity equation for such a probability distribution will then be

$$\frac{\partial \rho}{\partial t} + \frac{\partial}{\partial \phi}[\rho\dot{\phi}] + \frac{\partial}{\partial \omega}[\rho\dot{\omega}] = 0\,. \tag{32}$$

Here we take the usual Ott-Antonsen approach and rewrite the $\phi$ dependence of $\rho$ via a Fourier expansion, so that

$$\rho(\phi, \omega, \Omega; t) = \frac{W(\omega, \Omega; t)}{2\pi}\left[1 + \sum_n C_n(t) e^{in\phi} + C_n^*(t) e^{-in\phi}\right]. \tag{33}$$

where $W(\omega, \Omega; t)$ is the time-dependent marginal distribution after $\phi$ is integrated out. That is,

$$W(\omega, \Omega; t) = \int d\phi \rho(\phi, \omega, \Omega; t)\,. \tag{34}$$

Next we apply the Ott-Antonsen ansatz, which is to assume $C_n(t) = \alpha(t)^n$ for some complex-valued $\alpha(t)$. Putting this expression into the Fourier expansion and dropping the explicit time dependence of $\alpha$, we obtain

$$\rho(\phi, \omega, \Omega; t) = \frac{W(\omega, \Omega; t)}{2\pi}\left[1 + \sum_n (\alpha e^{i\phi})^n + ((\alpha e^{i\phi})^*)^n\right], \tag{35}$$

where

$$\alpha \equiv |\alpha| e^{-i\chi}\,. \tag{36}$$

Next we will plug this expression into our continuity equation, but first we simplify $\dot{\phi}$ and $\dot{\omega}$. In particular, the coupling term in the thermodynamic limit is

$$\frac{1}{N}\sum_j \sin(\phi_j - \phi_i) \to \int d\phi'\, d\omega\, d\Omega\ \rho(\phi', \omega, \Omega; t) \sin(\phi' - \phi)\,. \tag{37}$$

If we now plug in the definition of $\rho$ from Equation (33), as well as applying the Ott-Antonsen ansatz $C_n(t) = \alpha(t)^n$, we can evaluate the integral and obtain

$$\int d\phi'\, d\omega\, d\Omega\ \rho(\phi', \omega, \Omega; t) \sin(\phi' - \phi) = r \sin(\psi - \phi), \tag{38}$$

where

$$re^{i\psi} \equiv \mathscr{r} \equiv \int d\phi'\, d\omega\, d\Omega\ \rho(\phi', \omega, \Omega; t) e^{i\phi} = \int d\omega\, d\Omega\, \alpha^* W(\omega, \Omega)\,. \tag{39}$$

Thus, $\dot{\phi}$ and $\dot{\omega}$ simplify to

$$\dot{\phi} = \omega + Kr \sin(\psi - \phi) \tag{40}$$

and

$$\dot{\omega} = D(\Omega - \omega) + \beta K r \sin(\psi - \phi)\,. \tag{41}$$

Now we can plug this expression into our continuity equation. By orthogonality, we can separate the continuity equation into each power $e^{in\phi}$, though only $n = 0$

and $n = 1$ will give unique equations. These are quite complex, but we present them here. For $n = 0$, we obtain

$$\frac{\partial W}{\partial t} + \frac{\partial}{\partial \omega}\Big[W\big\{D(\Omega - \omega) + K\beta|\alpha| r \sin(\psi - \chi)\big\}\Big] = 0, \tag{42}$$

and for $n = 1$, we obtain

$$\begin{aligned} W\frac{\partial \alpha}{\partial t} &+ \left\{\frac{i}{2}\beta K \mathcal{r}^* \frac{\partial W}{\partial \omega} - \frac{1}{2}K\mathcal{r}^* W\right\} + \alpha\left\{i\omega W + D(\Omega - \omega)\frac{\partial W}{\partial \omega} - DW\right\} \\ &+ \alpha^2\left\{\frac{1}{2}K\mathcal{r}W - \frac{i}{2}\beta K\mathcal{r}\frac{\partial W}{\partial \omega}\right\} + \frac{\partial \alpha}{\partial \omega}\left\{D(\Omega - \omega)W\right\} \\ &+ \alpha\frac{\partial \alpha}{\partial \omega}\left\{-i\beta K\mathcal{r}W\right\} = 0\,. \end{aligned} \tag{43}$$

The first of these equations clearly governs the resource dynamics, while the second governs the phase dynamics. While the first equation is somewhat intuitive, the second is quite complicated. Thus, we will now consider an additional simplification. That is, we will assume the resource dynamics occur on a much slower timescale than the phase dynamics. We impose this condition by scaling all of the parameters in the following way: $K \to \Lambda K$, $\Omega \to \Lambda\Omega$, $D \to \Lambda^{-1}D$, $\beta \to \Lambda^{-1}\beta$, and $\omega \sim \mathcal{O}(\Lambda)$, where $\Lambda$ is some very large scalar. We will also separate the time variable into a fast time and a slow time by letting $t = \Lambda^{-1}\tau + T$, where $\tau$ is the fast timescale and $T$ is the slow timescale. We see this most clearly when looking at rates of change, for which the timescale separation gives $\frac{\partial}{\partial t} = \Lambda\frac{\partial}{\partial \tau} + \frac{\partial}{\partial T}$, so we see that rates of change on the fast timescale are very large compared to rates of change on the slow timescale. Now we plug this expression into our two differential equations and collect terms in powers of $\Lambda$. In doing this, we obtain 4 equations:

$$\frac{\partial W}{\partial \tau} = 0 \tag{44}$$

$$\frac{\partial \alpha}{\partial \tau} + \frac{K}{2}(\alpha^2\mathcal{r} - \mathcal{r}^*) + i\alpha(\Lambda^{-1}\omega) = 0 \tag{45}$$

$$\frac{\partial W}{\partial T} + \frac{\partial}{\partial \omega}\Big[W\big\{D(\Omega - \omega) + K\beta|\alpha| r \sin(\psi - \chi)\big\}\Big] = 0 \tag{46}$$

$$W\frac{\partial \alpha}{\partial T} + \frac{\partial}{\partial \omega}\Big[W\{\alpha D(\Omega - \omega) - \frac{i}{2}\beta K(\alpha^2\mathcal{r} - \mathcal{r}^*)\}\Big] = 0 \tag{47}$$

supplemented by the equation

$$\mathcal{r} = re^{i\psi} = \int d\Omega\, d\omega\, \alpha^*(\omega, \Omega; \tau, T)\, W(\omega, \Omega; T)\,. \tag{48}$$

There is one final detail, which is that we have not *quite* separated the timescales completely. In particular, the slow timescale equations contain terms depending on $\alpha$ and $\mathcal{r}$, both of which change on the fast timescale. However, since the

fast timescale dynamics are simply the *usual* Kuramoto dynamics, we can take advantage of the fact that for the usual Kuramoto dynamics, all dynamics move to stable fixed points, rather than any sort of cycle. Thus, we can exploit the timescale separation by assuming that, on the slow timescale, all dynamics on the fast timescale have already equilibrated to their respective fixed points. Unfortunately, here we run into a significant problem. We do not know, for an arbitrary frequency distribution $W$, what the equilibrium order parameter will be. In fact, there are in some cases multiple fixed points for the order parameter, so the solution is not even unique. Thus, at this point our analytic efforts halt, and this is why all argument in the paper is left intuitive, rather than mathematically deductive.

# 7 Dynamics When $\Lambda \ll 1$

In Figure 3 we give a sample plot of $\Lambda \ll 1$ for the "bistable" configuration where $\beta > 0$. We can clearly see that the seemingly first-order transition has vanished in this limit, as has any appreciable hysteresis. This behavior demonstrates that in the limit of small $\Lambda$, we simply obtain the usual Kuramoto dynamics, as we would intuitively expect from our description of the model as "resource-constrained".

# 8 Behavior of $\Omega(t)$

One may wonder what the behavior of the group velocity of the system is. Define this group velocity, $\Omega(t)$ to be simply the average velocity of all of the oscillators in the system. That is,

$$\Omega(t) = \frac{1}{N} \sum_j \omega_j(t) \tag{49}$$

We are interested in the time-dependence of this quantity, so we take the time derivative, giving

$$\dot{\Omega}(t) = \frac{1}{N} \sum_j \dot{\omega}_j(t) \tag{50}$$

From here, we may substitute in our equation for $\omega_j(t)$, giving

$$\dot{\Omega}(t) = \frac{1}{N} \sum_j \left[ D(W_j - \omega_j) + \beta \frac{K}{N} \sum_i A_{ij} \sin(\phi_j - \phi_i) \right] \tag{51}$$

Now since $A_{ij}$ is assumed to be an undirected graph, it will be symmetric under interchange of $i$ and $j$. Meanwhile, the sine term will be antisymmetric under such an interchange. Thus, summing over both $i$ and $j$ will evaluate precisely to zero, so we can drop the second term altogether, leaving only

$$\dot{\Omega}(t) = \frac{1}{N} \sum_j D(W_j - \omega_j) \tag{52}$$

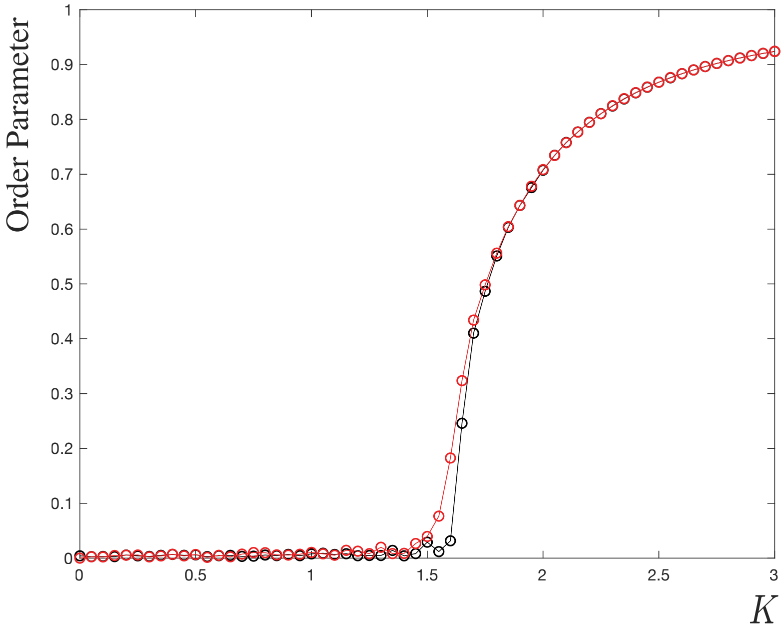


Figure 3: **Phase Transition for $\mathbf{\Lambda \ll 1}$ and $\beta > \mathbf{0}$**. The black curve gives the upward-going transition to order, while the red curve gives the downward-going transition to disorder.

We can now break the sum over the two terms, giving

$$\dot{\Omega}(t) = D\Big[\frac{1}{N}\sum_j W_j - \frac{1}{N}\sum_j \omega_j\Big] \tag{53}$$

The first term gives the average of $W_i$, which is just some constant, while the second term is the definition of $\Omega$. Thus,

$$\dot{\Omega}(t) = D\big(\langle W\rangle - \Omega\big) \tag{54}$$

This is clearly just diffusion dynamics, so the solution for $\Omega(t)$ will be simply

$$\Omega(t) = (\Omega_0 - \langle W\rangle)e^{-Dt} + \langle W\rangle \tag{55}$$

where $\Omega_0$ is just the initial average frequency of the system.
This time-dependence is not impacted by any of the synchronization dynamics occurring in the system since all of the Kuramoto interactions are antisymmetric, and therefore zero on average over the entire system.

# 9 Possibility of Travelling Waves

Related to the above, one might wonder whether travelling waves may appear in this system, as they have in other Kuramoto systems. There are two distinct types of travelling waves. One may be found even in the standard Kuramoto model. For example, Pazo and Montbrio show in their 2009 paper "Existence of hysteresis in the Kuramoto model with bimodal frequency distributions" that if a frequency distribution is sufficiently bimodal, a standing wave state appears; that is, two travelling waves move with equal speeds in opposite directions.
However, there is another travelling wave state that has been observed only in modified Kuramoto models. In particular, Strogatz and Hong (2011) observe that by allowing some oscillators in the system to have negative couplings, non-symmetric travelling wave states may appear. We do not have any reason to believe that the model proposed here could produce a travelling wave state in the same sense. This is because such states appear to require that the Kuramoto coupling no longer be zero on average. That is, we have relied on the fact that $K$ be the same for all oscillators (and that the connection graph be undirected), because this allows

$$\sum_i K \sum_j A_{ij}\sin(\phi_j - \phi_i) = 0 \tag{56}$$

However, in the Strogatz and Hong paper, some oscillators have coupling $K$ and some have coupling $-K$. That is, $K = K_i$, where $K_i = \pm K$, depending on the oscillator $i$. This will break the clean symmetries that allow the above equality. That is, suppose there are only two oscillators and that one is coupled positively while the other is coupled negatively. Then the above summation becomes

$$K\sin(\phi_1 - \phi_2) + (-K)\sin(\phi_2 - \phi_1) = 2K\sin(\phi_1 - \phi_2) \neq 0 \tag{57}$$

This broken symmetry seems to be important for the existence of asymmetric travelling wave states, and since the symmetry is unbroken in the model considered here, we believe such states will not be allowed.
